# Supplementary material for: Atomic resolution observations of silver segregation in a [111] tilt grain boundary in copper
Source: arXiv:2212.01180 ancillary file (2022-12-02)
Supplement: Supplementary file 1 [file supplementary-information.pdf]

*Supplementary Data*

# Atomic resolution observations of silver segregation in a [111] tilt grain boundary in copper

Lena Frommeyer, Tobias Brink,
Gerhard Dehm, and Christian H. Liebscher

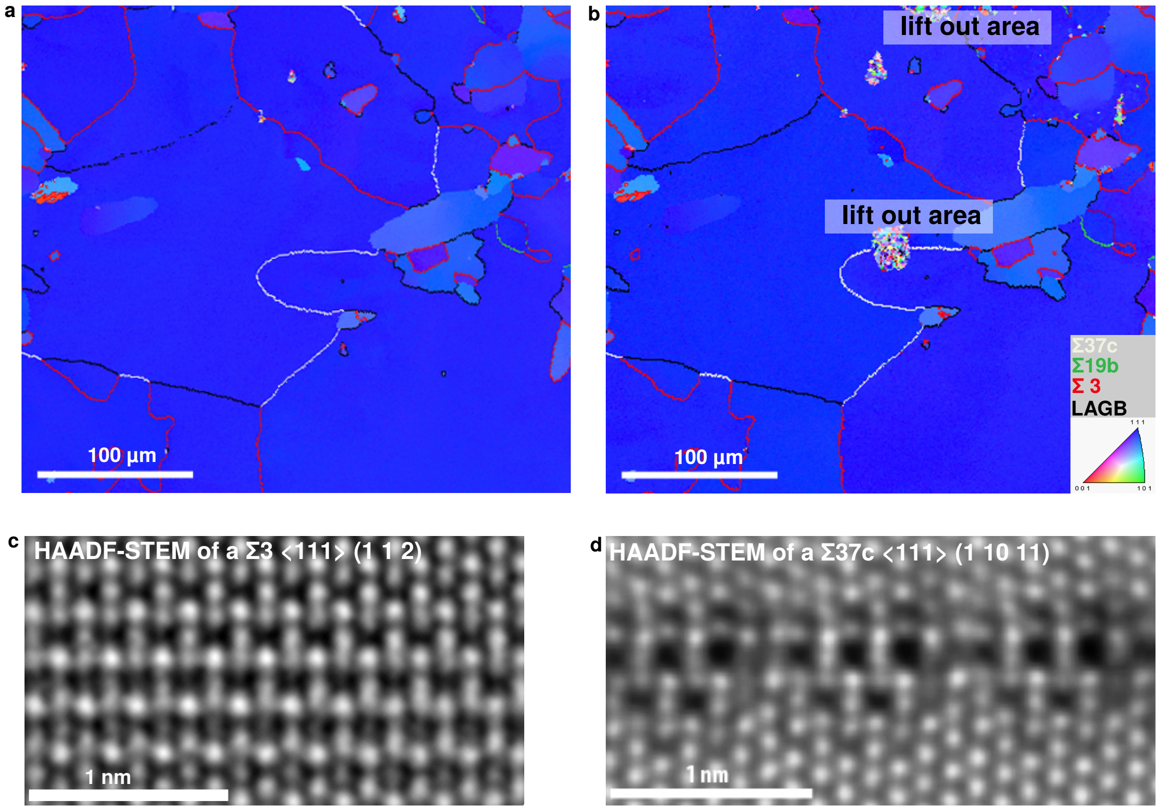


**Figure S1:** Comparison of the same area in the pure Cu film before (a) and after (b) annealing at 600°C for 16 h. In (b), the lift out areas are visible which were used for investigating the pure Cu $\Sigma$ 37c $\langle 111 \rangle \{347\}$ GB before annealing. (c) shows a HAADF-STEM image of a $\Sigma$ 3 $\langle 111 \rangle \{112\}$ GB in pure Cu, which consists of only squares. (d) is a HAADF-STEM image of a $\Sigma$ 37c $\langle 111 \rangle \{347\}$ of the pure Cu film without Ag after annealing which is shown in (b). It shows the same GB structure as prior to annealing or annealing with Ag (Fig.2).

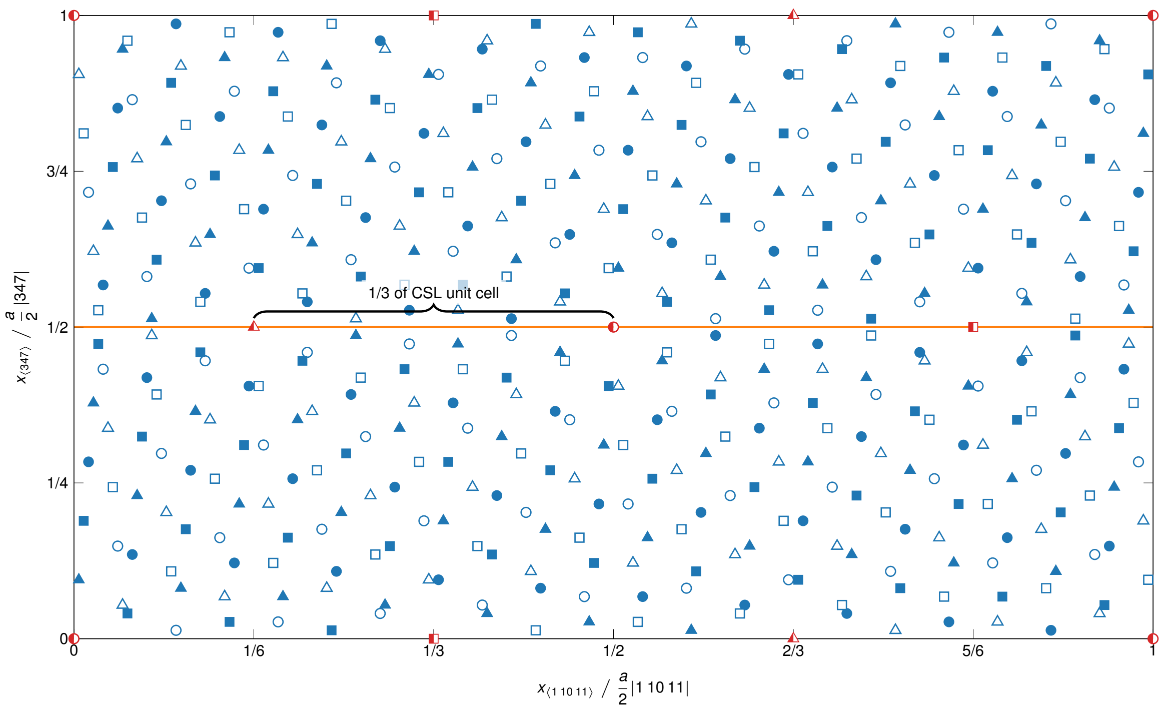


**Figure S2:** Dichromatic pattern of the Σ37c GB. The filled and unfilled dots are belonging to the two different grains. The different shapes show different z-heights in the unit cell. The black line indicates the {347} GB plane.

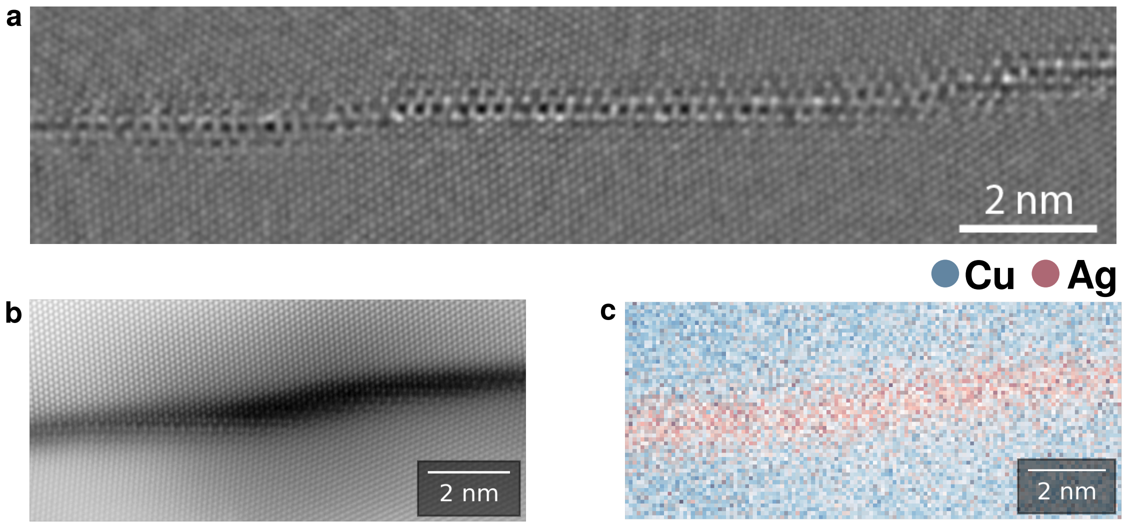


**Figure S3:** Asymmetric areas of the Σ37c ⟨111⟩ zipper structure. a) HAADF-STEM showing an asymmetric structure. The asymmetry is compensated by "steps" of the GB. b) HAADF-STEM image of the area in which an Energy dispersive X-ray spectroscopy map was registered with a high voltage of 300 kV. c) Intensity map of the Cu K$\alpha$ peak (blue) and Ag L$\alpha$ peak (red). Ag is enriched at the GB, however no enrichment could be observed at the steps of the GB.

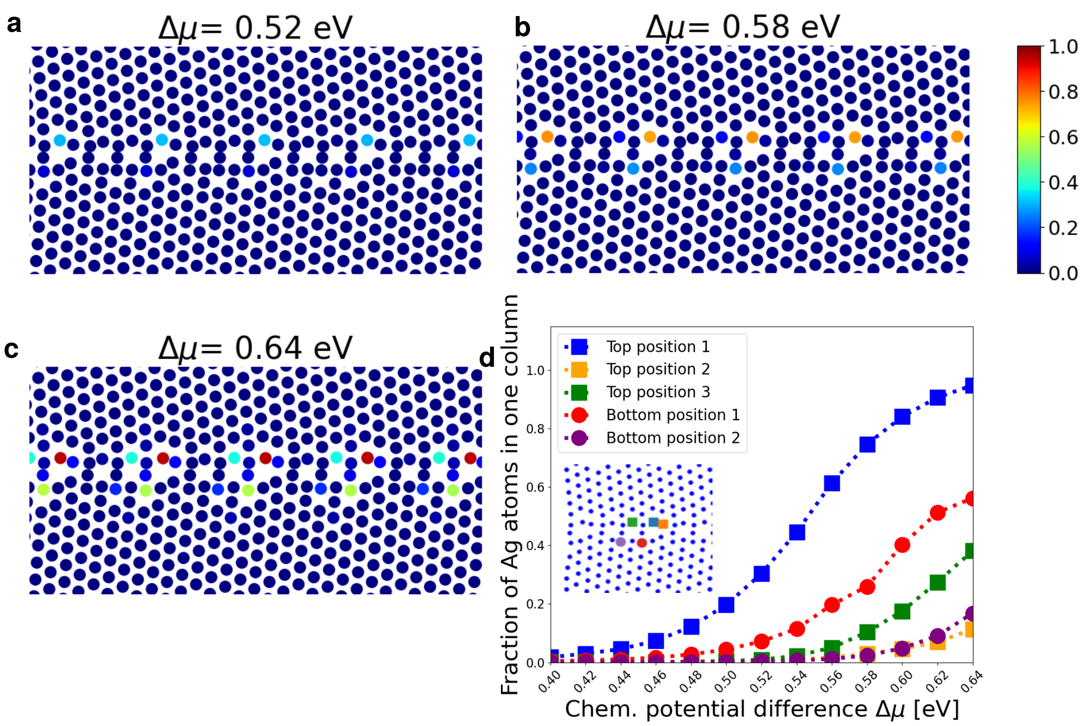


**Figure S4:** Ag occupancy of the columns by increasing the chemical potential at 500K. All simulations were equilibrated.

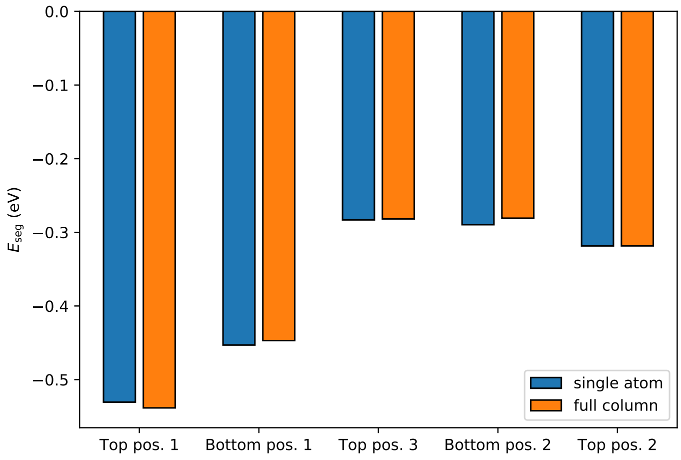


**Figure S5:** Segregation energies for Ag on the different positions in the GB. The segregation energies were calculated once with one silver atom in a box with 15 periodic images along the tilt axis direction and once with fully silver-filled columns. The energy differences between these two cases are very small.

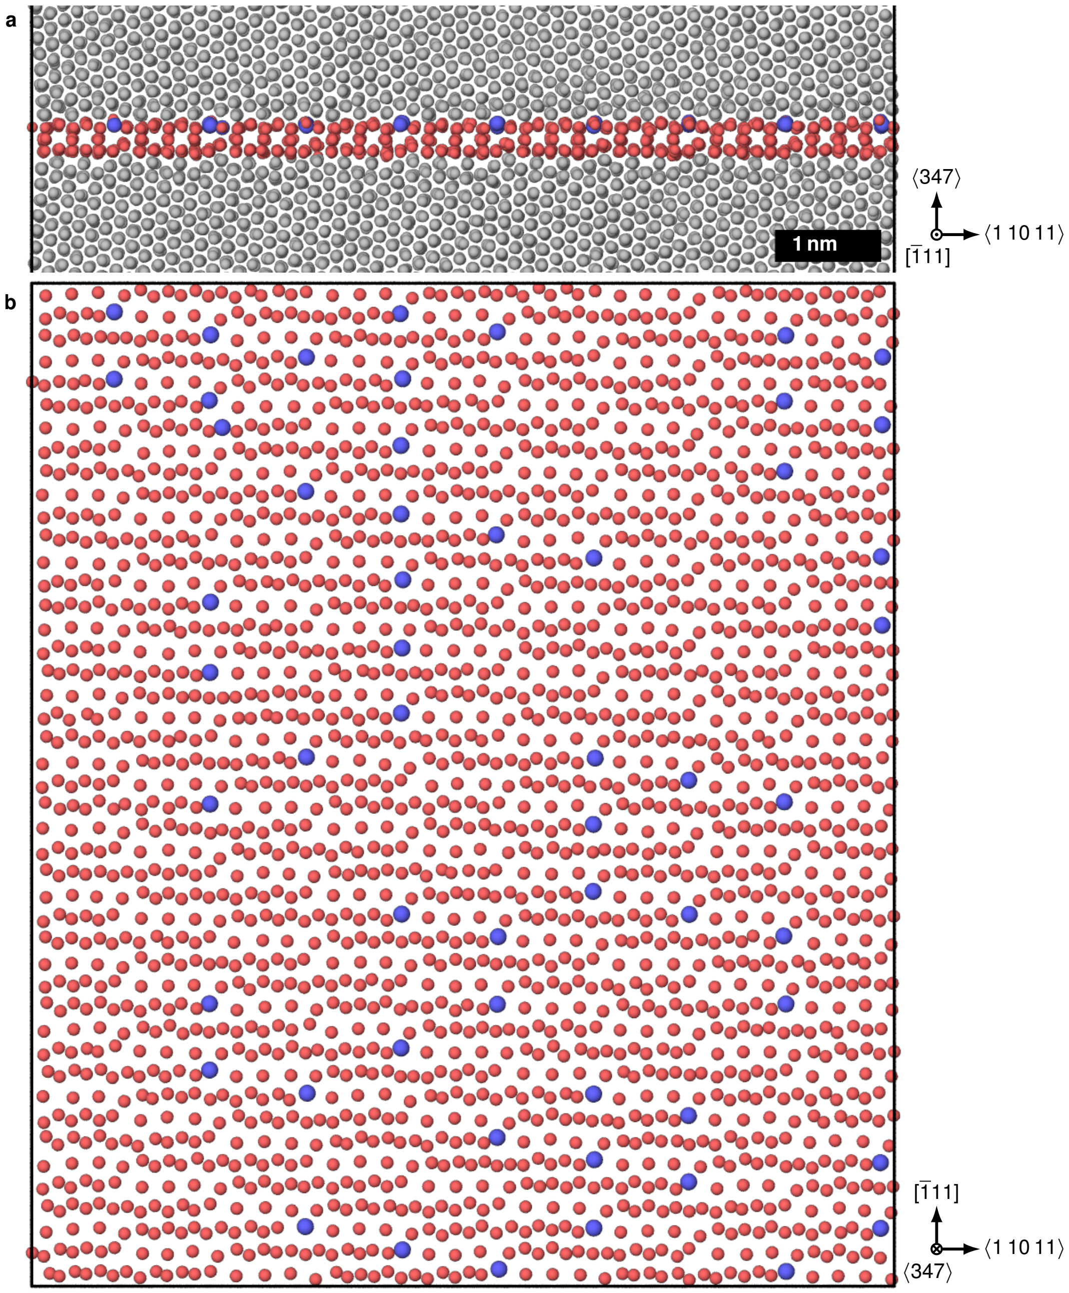


**Figure S6:** Snapshot of the GB with $\Delta\mu = 0.54\,\text{eV}$, where top position 1 is approximately half filled. (a) View along the [$\bar{1}$11] tilt axis. Bulk atoms are colored in gray, GB atoms in red if they are Cu atoms and in blue if they are Ag atoms. The Ag atoms are visualized with larger spheres to make them easier to discern. Black lines indicate the periodic boundaries of the simulations cell. (b) Cross-sectional view, with the gray bulk atoms removed. The silver atoms are randomly distributed, which fits the fact that the segregation energies are similar for isolated atoms and filled columns (Supplemental Fig. S5).

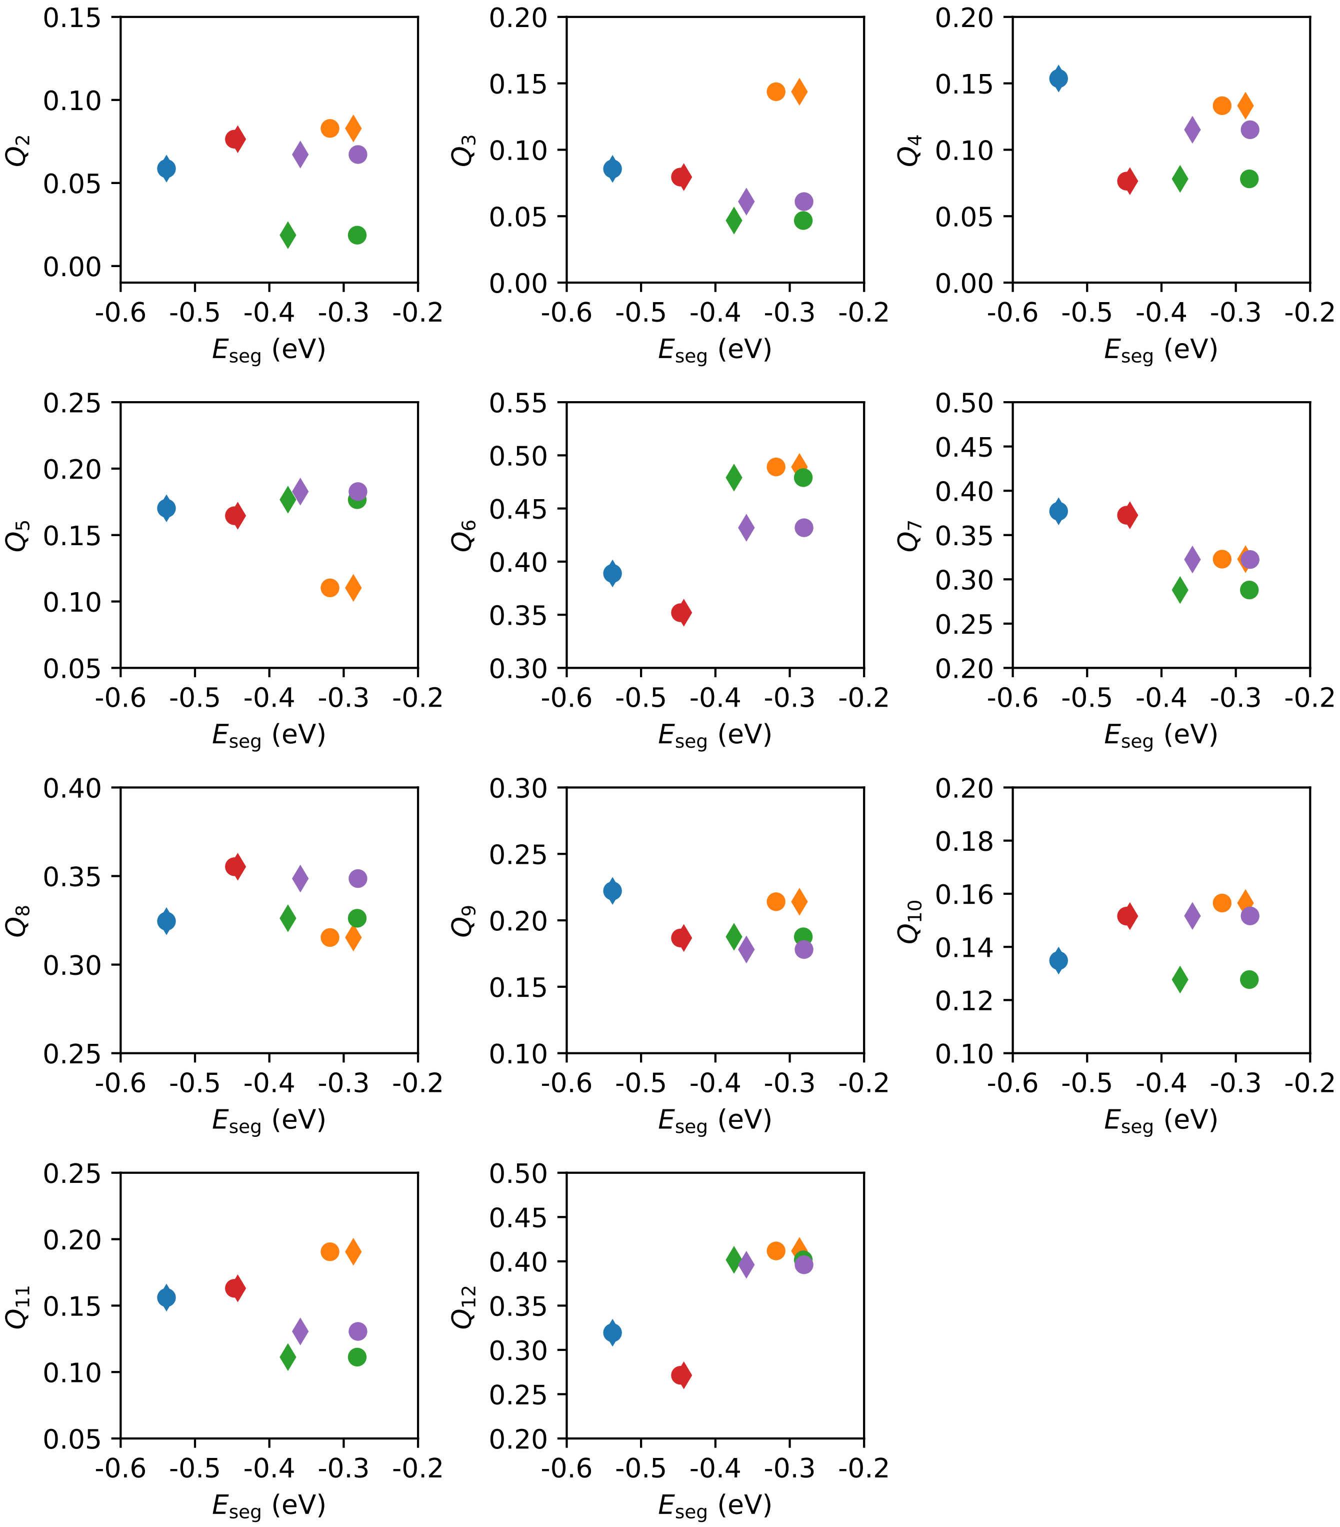


**Figure S7:** Steinhardt parameters of the GBs atoms in the columns where Ag substitution takes place. No clear correlation between any of these local, structural parameters and the segregation energy can be observed.
